# Supplementary material for: Data-Agnostic Augmentations for Unknown Variations: Out-of-Distribution Generalisation in MRI Segmentation
Source: arXiv:2505.10223 source file (2025-05-15)
Supplement: Supplementary file 1 [file quali_segmentation_map.tex]

% Fig.~\ref{fig:example_predictions} visualizes the effect of using base, MixUp, and AFA augmentations on the transformed test set. Notably, while intensity shift augmentation is among the base augmentations, the top row shows that AFA and MixUp are required to correct for the bias field in the data.

% \begin{figure}[!tbh]
%     \centering
%     \includegraphics[width=0.9\linewidth]{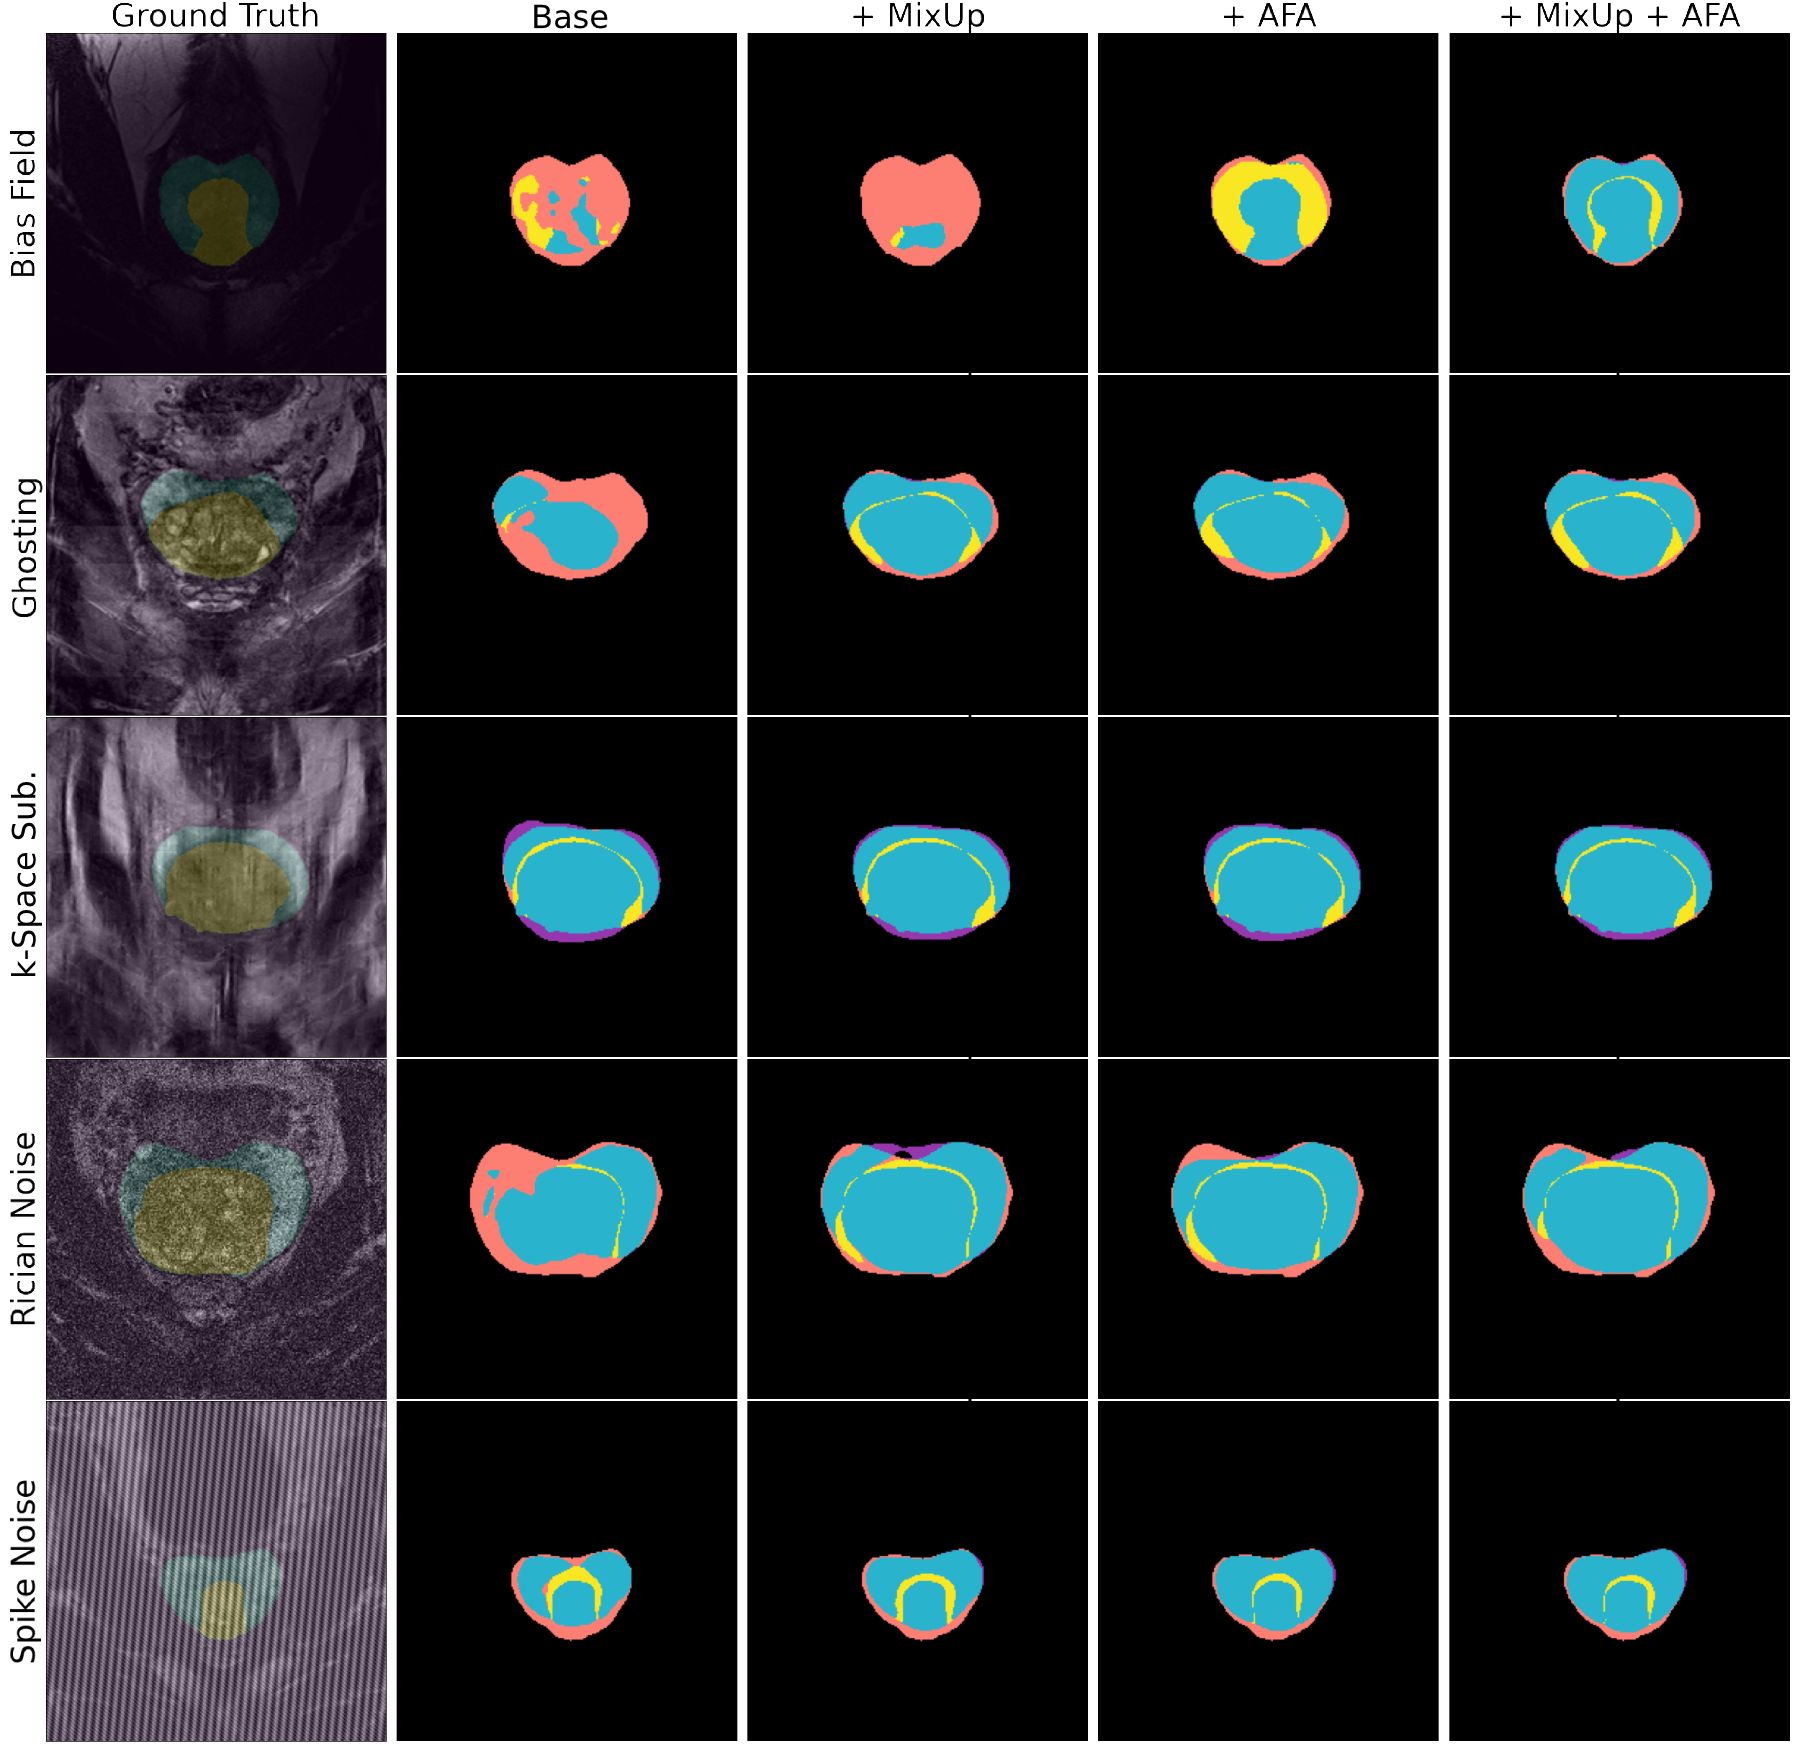}
% \begin{tikzpicture}
% \definecolor{correct}{RGB}{42, 179, 205}
% \definecolor{missclassification}{RGB}{250, 231, 35}
% \definecolor{undersegmentation}{RGB}{253, 127, 116}
% \definecolor{oversegmentation}{RGB}{150, 55, 173}
%     \begin{customlegend}[legend columns=-1,legend style={draw=none,column sep=1ex},legend entries={\scriptsize Correct, \scriptsize Under Segmentation, \scriptsize Misclassification, \scriptsize Over Segmentation}]
%     \addlegendimage{area legend,color=correct,fill}
%     \addlegendimage{area legend,color=undersegmentation,fill}
%     \addlegendimage{area legend,color=missclassification,fill}
%     \addlegendimage{area legend,color=oversegmentation,fill}
%     \end{customlegend}
% \end{tikzpicture}%
%     \caption{In the first column, we show the ground truth with the expert annotated mask and in the following columns, we show the model predictions made by nnU-Net with augmentations, alone or in combination with MixUp and/or AFA. In presence of AFA and/or MixUp we see a substantial improvement in segmentation coverage under difficult imaging conditions.}
%     \label{fig:example_predictions}
% \end{figure}
