# Supplementary material for: Data-Agnostic Augmentations for Unknown Variations: Out-of-Distribution Generalisation in MRI Segmentation
Source: arXiv:2505.10223 source file (2025-05-15)
Supplement: Supplementary file 2 [file calibration.tex]

\begin{table}[!tbh]
    \centering
    \caption{\newtext{The expected calibration error for the validation set of the dataset ACDC and P158.}}
    \label{tab:my_label}
    \input{tables/calibration/ece}
\end{table}
