# Supplementary material for: Data-Agnostic Augmentations for Unknown Variations: Out-of-Distribution Generalisation in MRI Segmentation
Source: arXiv:2505.10223 source file (2025-05-15)
Supplement: Supplementary file 3 [file avg_metrics_supp_ds.tex]

\resizebox{\textwidth}{!}{%
\begin{tabular}{ccccccccc}
\toprule
\multicolumn{3}{c}{Augmentation}          & \multicolumn{3}{c}{Cardiac Cine MR} & \multicolumn{3}{c}{Prostate bpMRI} \\ \cmidrule{1-3} \cmidrule(lr){4-6} \cmidrule(lr){7-9}
nnUNet       & MixUp        & AFA          & Trained On   & DSC     & HD95 (mm)   & Trained On   & DSC    & HD95 (mm)  \\ \midrule
$\checkmark$ &              &              & \multirow{4}{*}{ACDC}         & 0.870   & 7.97        &  \multirow{4}{*}{MSD}         & 0.653  & 10.14      \\
$\checkmark$ & $\checkmark$ &              &                        & {\color[HTML]{3233B9} 0.880} & {\color[HTML]{3233B9} 5.74} &                       & {\color[HTML]{3233B9} 0.705} & {\color[HTML]{3233B9} 9.29} \\
$\checkmark$ &              & $\checkmark$ &                        & {0.874} & {6.92} &                       & {\color[HTML]{3233B9} 0.706} & {\color[HTML]{3233B9} 9.39} \\
$\checkmark$ & $\checkmark$ & $\checkmark$ & \multirow{-4}{*}{ACDC} & {\color[HTML]{3233B9} 0.880} & {\color[HTML]{3233B9} 5.70} & \multirow{-4}{*}{MSD} & {\color[HTML]{3233B9} 0.695} & {\color[HTML]{3233B9} 9.60} \\ \midrule
$\checkmark^\dagger$ &              &              & M\&Ms        & 0.882   & 5.08        & P158         & 0.825  & 4.60       \\ \bottomrule
\end{tabular}
}
